# Supplementary material for: Aleph Filter: To Infinity in Constant Time
Source: arXiv:2404.04703 source file (2024-10-31)
Supplement: Supplementary file 1 [file appendices.tex]

\newpage

\section{Journal Extension }

\Paragraph{Knowing the Data Size In Advance} If we do know the maximum data size in advance, we can pre-allocate bits and then decrease out budget slowly. The point is that the log log N overhead needed for expansion can be paid upfront. 

\Paragraph{In-Between Design Option} Rather than allocating 2 * log log N new bits per entry, we can allocate  log log N. This causes the FPR to increase as log log N rather than be constant. However, this is still a reasonable design with significantly lower memory footprint, and a hardly increasing FPR. So it's a nice viable point in the space. 

\Paragraph{Adaptivity} If many Rejuvenation operations happen, we do not need to increase the memory footprint to stabalize the FPR. We should only increase it adaptively if no rejuvenations happen. 

\Paragraph{Non-Power of 2} We should be able to set the filter to a non-power of 2, and expand by other factors than 2. For example, we may want to expand by 4 times to amortize write cost, or we may want to expand by 1.5 to save space. It's a part of a trade-off continuum. 

\Paragraph{Ring Filters} Two papers still need to be referenced. ``The Consistent Cuckoo Filter'' and ``Towards Capacity-adjustable and Scalable Quotient Filter Design for Packet Classification in Software-Defined Networks''. Both filters create a hash rings, which can expand one fragment at a time. I read the latter and its analysis is very unpromising. A ring takes $O(\log N)$ time for queries, inserts and deletes, as the different nodes are organized in a binary search tree. But in fact, in the latter paper, when one ring fills up, they create an additional ring, which is presumably larger (though they don't say by how much). Let's assume the new ring is larger by a factor of 2, meaning we have information about one additional bit of each key's hash when its inserted. Our query/delete time is now $O(\log(N)^2)$. The paper says they try to insert elements to whichever ring has the fewest elements, but this implies inserting from smallest to largest rings and implies insertion time of $O(\log(N)^2)$ as well. And the FPR is proportional to the number of rings, so should be $O(\log N)$. Overall this is totally noncompetitive. Need to check the consistent cuckoo filter again. 

\section{Appendices}

\begin{table*}
	\footnotesize
	\begin{tabular}{ |p{2.5cm}|p{1.8cm}|p{2.3cm}|p{1.9cm}|p{2.3cm}|p{1.6cm}|p{1.4cm}|p{2.2cm}|}  
		%\begin{tabular}{ |l c c c c|  }
		%\hline
		%\multicolumn{4}{|c|}{Country List} \\
		\hline
		InfiniFilter (IF) type & query / delete& insert & false positive rate & fingerprint \newline bits / entry & maximum \newline expansions & data \newline retrievals & limitations \\
		\hline
		Basic IF 	  		 								    & $O(1)$  & $O(1)$ 	&  $O(2^{-F}   \cdot \lg N_K )$ &   $F$  & $F$ & 0 &  \\
		Basic IF 	\& Poly. FPRs    		 		   & $O(1)$  & $O(1)$ 	&  $O(2^{-F}   )$ &   $F + O( \lg \lg N) $  & $F $ & 0 & \\
		Chained IF   		 								& $O(\frac{\lg N}{F})$  & $O(1)$ 	&  $  O(2^{-F}   \cdot \lg N )$ &   $F$  & $\infty$  & 0 & \\
		Chained IF  \& Poly. FPRs 				 & $O(\frac{\lg N}{F + \lg \lg N})$??  & $O(1)$	&  $O(2^{-F} ) $ &  $F+ O(\lg \lg N)$  & $\infty$  & 0 & \\
		Chained IF  \& Exp. FPRs 				 & $O(\frac{\lg N}{F + \lg N})$??  & $O(1)$	&  $O(2^{-F} ) $ &  $F + O( \lg N)$  & $\infty$  & 0 & \\
		%Basic IF 	\& Exp. FPRs    		 		   & $O(1)$  & $O(1)$ 	&  $O(\varepsilon \cdot \frac{\lg N}{N}  )$ &   $O(\lg \nicefrac{1}{\varepsilon} + \lg N) $  &  $\infty$ & 0 & \\
		Duplic. IF   		 			  					& $O(1)$  & $O( (0.5 - 2^{-F} \cdot \lg N)^{-1} )$ 	&  $O(2^{-F}  \cdot \lg N )$ &   $F$  & $O(2^F)$  & 0 &  deletes need ages \\
		Duplic. IF  \& Poly. FPRs  		  		& $O(1)$  & $O(1)$ &  $O(2^{-F}  )$ &   $F + O(\lg \lg N)$  & $\infty$  & 0 & deletes need ages    \\
		Reinserting IF 	  		 						& $O(1)$  & $O(1)$ 	&  $O(2^{-F}   )$ &   $F$  & $\infty$  & $O(2^{-F} \cdot N)$ & one-to-one map  \\
		
		%7. Goal   						 																				   & $O(1)$ 			&  $O(1)$ &  $O(1)$ & $O(\varepsilon  )$&    $O(\lg \nicefrac{1}{\varepsilon})$ & $\infty$ & 0 \\
		\hline
	\end{tabular}
	\caption{A comparison of different techniques for expanding a Filter. As shown, no existing method for filter expansion allows to achieve perfect scalability with data size for queries, inserts, deletes, the false positive rate and the memory footprint at the same time. Can we achieve the best of all worlds, as shown in the last row?   } \label{tab:infini}
\end{table*}

\section{Notes} \label{sec:intro}

\begin{enumerate}
	\item In Chucky, there could be multiple entries with the same key at different levels of the LSM-tree. We needed to map them to the same pair of cuckoo buckets to keep access time low. To do this, we assign all a minimum fingerprint size, and we swap them in the filter based on this minimum fingerprint size. This is why we couldn't use Cuckoo filter. It would force us to look at the original data when expanding for entries with the minimum fingerprint size. So Cuckoo filter would allow mitigating the expansion problem, but not eliminating it. The reason is that it uses fingerprints as a part of the conflict resolution mechanism. 
	\item We can insert the same key multiple times. This will create multiple hash entries within the same hash bucket. The only caveat is it seems we can only delete an entry. 
\end{enumerate}

Handling Deletes in EQF. Do we ever need to read the original data to handle a delete? Let's assume here no rebirth operations. Theory: assuming we always delete an entry that has actually been inserted, as long as we delete the entry with the greatest matching fingerprint, we can handle the delete without looking at the original data.

\begin{enumerate}
	\item suppose we have two fingerprints in the same run of  the second newest and newest generations, respectively: 01 0000 and 1 01010. Suppose they correspond to entries Y and X, respectively. We can delete either one of them without looking at the original data. 
	\item suppose we have two fingerprints in the same run of the second newest and newest generations, respectively: 01 0101 and 1 01010. Suppose they correspond to the same entry X. When we make a delete operation, we get rid of the longest match from the newest generation. 
	\item  suppose we have two fingerprints in the same run the second newest and newest generations, respectively: 01 0101 and 1 01010. Suppose they correspond to entries Y and X, respectively, and that the full fingerprint of Y is 01011 (different from X). When we make a delete operation of X, if we were to delete the shorter matching fingerprint, we would get a false negative in the future when querying for Y. 
	\item We always employ the same hash function. It's just that as the filter grows, we maintain more bits of this hash since the slot address we need is longer (while the initial fingerprint size is always the same). 
	\item Pedro: For positive queries, the FPR can be reduced: if we get say two matches we should try them in the order of their fingerprint lengths. This may help reduce the effective FPR seen for positive lookups due to old entries with shorter fingerprints which may have a meaningful benefit for workloads on which positives dominate.
	
\end{enumerate}

How to handle rebirth operations? Find the entry in the run with the greatest matching fingerprint. Expand it. 

Delete operations in conjunction with insertions can be used to easily implement rebirth operations.

\section{The Exponential Quotient InfiniFilter} \label{sec:reinserting}

\Paragraph{Retrieval} After several expansions, some entries may no longer have fingerprints. We read them from storage and reinsert them. The worst-case overhead is $O(N \cdot \varepsilon)$, though in practice is can be substantially eliminated as we see next. This is useful under three assumptions about the application: (1) storage mimics the filter organization  so we can find entries. This is for instance true in networking. (2) We have physical pointers to data entries. (3) If we have no deletes and storage is append-only, we can just look at oldest data. 

\section{Calculations for the Chained InfiniFilter with Poly Fingerprints}
\begin{align} 
	\theta_0  &= \sum_{i=0}^{X}  {f(X, i)}  \cdot 2^{-FP_0(X,i)} \nonumber\\
	&=  \sum_{i=0}^{X-1}  2^{-i-1}  \cdot 2^{-F - 2 \cdot \log_2(X-i) + i} + 2^{-X} \cdot 2^{-F + X} \nonumber \\
	& =  2^{-F-1}\cdot\sum_{i=0}^{X-1}   2^{ - 2 \cdot \log_2(X-i)} + 2^{-F} \nonumber \\
	& =  2^{-F-1}\cdot\sum_{i=0}^{X-1}   \frac{1}{(X-i)^2} + 2^{-F} \nonumber\\
	&\leq2^{-F}\cdot \frac{3}{2}\cdot  \sum_{i=1}^{X}   \frac{1}{i^2}   \label{eq:FPR1-poly}
\end{align}

For $a>0$, we get that the false positive rate is:

\begin{align} 
	\theta_a  &= \sum_{i=0}^{X}  {f(X, i)}  \cdot 2^{-FP_a(X,i)} \nonumber\\
	&=  \sum_{i=0}^{X-1}  2^{-i-1}  \cdot 2^{-F - 2 \cdot \log_2(a+X-i) + i} + 2^{-X} \cdot 2^{-F - 2 \cdot \log_2(a)+ X} \nonumber \\
	& =  2^{-F-1}\cdot\sum_{i=0}^{X-1}   2^{ - 2 \cdot \log_2(a+X-i)} + 2^{-F} \cdot 2^{- 2 \cdot \log_2(a)} \nonumber \\
	& =  2^{-F-1}\cdot\sum_{i=0}^{X-1}   \frac{1}{(a+X-i)^2} + 2^{-F} \cdot \frac{1}{a^2} \nonumber\\
	&\leq2^{-F}\cdot\sum_{i=0}^{X}   \frac{1}{(a+i)^2}   \label{eq:FPR2-poly}
\end{align}
